# Supplementary material for: A Semantic Framework for the Security Analysis of Ethereum smart contracts
Source: arXiv:1802.08660 source file (2018-04-23)
Supplement: Supplementary file 1 [file appendix.tex]

\subsection{Transactions}
Formally, a transaction is a tuple $(\transactionnonce, \gasprize, \allowbreak \gaslimit, \allowbreak \recipient, \allowbreak \transactionvalue, \allowbreak \sender, \allowbreak \transactioninput, \transactiontype)$ 
where 
\begin{itemize}
\item 
$\transactionnonce$ is a number counting the number of transactions issued by the sender
\item 
$\gasprize$ is the amount of ether to pay for one unit of gas when executing this transaction
\item 
$\gaslimit$ is the maximum amount of gas to be spent on the execution of the transaction 
\item 
$\recipient$ is the recipient of the the transaction 
\item 
$\transactionvalue$ is the amount of {$\wei$} transferred by the transaction 
\item 
$\sender$ is the sender of the transaction 
%TODO note that this actually is not the sender but information to identify the sender 
\item 
$\transactioninput$ is the input given to the transaction. This might either be the arguments given to a contract in case of a call transaction or the byte code that initializes the newly created contract in the case of a create transaction
\item 
$\transactiontype$ is the type of the transaction which is either a call or a create transaction. 
%TODO make the set explicit 
\end{itemize}
%TODO actually we would need to include the suicide set so that we can model the effect of a whole transaction 

A transaction not only causes byte code to be executed, but additionally includes some initialization and finalization steps that together with the effects of the code execution determines the effects of the transaction on the global state of the system. 

\subsection{Small step semantics}

We define a relation of the form $\sstep{\transenv}{\callstack}{\callstack'}$ where $\transenv$ is the transaction environment and $\callstack$ and $\callstack'$ denote call stacks of the execution. 
The transaction environment contains the parameters of the transaction that can be accessed by the code during execution, but can not be altered. In particular $\transenv$ contains the following information: 
\begin{itemize}
\item the address $\originator$ of the account that made the transaction
\item the gas prize $\gasprize$ for the transaction that specifies the amount of {wei} to pay for a unit of gas
\item the block header $\blockheader$ of the block the transaction is executed in 
\end{itemize}

%TODO add types 
A block header is of the form  $(\parent,$ $\beneficiary,$ $\difficulty,$  $\blocknumber,$ $\gaslimit,$ $\timestamp)$. 
Where $\parent$ identifies the header of the block's parent block, $\beneficiary$ is the address of the beneficiary of the transaction, $\difficulty$ is a measure of the difficulty of solving the proof of work puzzle required to mine the block, $\blocknumber$ is the number of ancestor blocks, $\gaslimit$ is the maximum amount of gas that might be consumed when executing the blocks transactions and $\timestamp$ is the Unix time stamp at the block's inception.  %TODO maybe we can omit this paragraph as this part of the formalization is not needed for understanding the paper 

\section{Content from previous definitions}

As for our definitions, we are only considered in parts of the traces produced by the execution, we assume projection functions that filter only specific actions of a trace: 
\begin{definition}[Projection on execution traces]
	Let $f \in \actions \to \BB$ be a filtering function. Then the projection on traces is recursively defined as follows
	\begin{align*}
	\project{\pi}{f} =
	\begin{cases}
	\nil & \pi = \nil \\
	\cons{a}{(\project{\pi'}{f})} & \pi = \cons{a}{\pi'} \land f(a) = 1  \\
	\project{\pi'}{f} & \pi = \cons{a}{\pi'} \land f(a) = 0
	\end{cases}
	\end{align*}
\end{definition}

In the following, let $\filtercallscreates{c}$ denote the function filtering all call and create actions of contract $c$: 
\begin{align*}
\filtercallscreates{c}(a) = 
\begin{cases}
1 & a = \CALL_{c}(g, \recipient, \valu, \io, \is, \oo, \os) \\
& ~\lor~ a = \CREATE_{c}(\valu, \io, \is) \\
& ~\lor~ a = \CALLCODE_{c}(g, \recipient, \valu, \io, \is, \oo, \os) \\
& ~\lor~ a = \DELEGATECALL_{c}(g, \recipient,  \io, \is, \oo, \os) \\
& \text{for some } g, \recipient, \valu, \io, \is, \oo, \os \in \word \\
0 & \text{otherwise}
\end{cases}
\end{align*}

We define a function for updating the components of the global state and also lift it to an update function on execution states. 

\begin{definition}[Strong updates on global state]
	Let the function $\strongpartialupdategstate{\cdot}{\cdot} \in \gstates \allowbreak \times (\addresses \to (\NN \to \NN) \times (\NN \to \NN) \times ((\BB^{256} \to \BB^{256}) \to (\BB^{256} \to \BB^{256}) ) \allowbreak \times (\arrayof{\BB}\to \arrayof{\BB})) \to \gstates$
	%Function that updates just a fraction of the global state. 
	be defined as follows:
	\begin{align*}
	\strongpartialupdategstate{\gstate}{u} = 
	\lambda a. 
	(\nonceupdate(n), \balanceupdate(b), \storageupdate(\textit{s}),  \codeupdate(\textit{c}) ) 
	\end{align*}
	given
	$u(a) = (\nonceupdate, \balanceupdate, \storageupdate, \codeupdate)$
	and $\gstate(a) = \accountstate{n}{b}{s}{c}$
\end{definition}

We say that a strong update does not affect a component of the global state (for a certain address) if the update $u$ maps (this address) for this component to the identity function. 

Using this, we can easily express the partial update of contract codes in the global state in the execution states. 

\begin{definition}[Code updates in execution states]
	Let the function $\updatecodeexstate{\cdot}{\cdot} \in  \exstates \times (\addresses \pto \arrayof{\BB}) \to \exstates$ be defined as follows: 
	\begin{align*}
	\updatecodeexstate{s}{\codeupdates} = 
	\begin{cases}
	\regstate{\mstate}{\exenv}{\strongpartialupdategstate{\gstate}{u}} & s = \regstate{\mstate}{\exenv}{\gstate} \\
	s & \text{otherwise}
	\end{cases} 
	\end{align*}
	with
	\begin{align*}
	u = \lambda a. 
	\begin{cases}
	(\idfun{\NN}, \idfun{\NN}, \idfun{\BB^{256} \to \BB^{256}}, \lambda b. \codeupdates(a))  &  a \in \domain{\codeupdates} \\
	(\idfun{\NN}, \idfun{\NN}, \idfun{\BB^{256} \to \BB^{256}}, \idfun{\arrayof{\BB}}) & \text{otherwise}
	\end{cases}
	\end{align*}
	
	and $\idfun{\NN}$, $\idfun{(\BB^{256} \to \BB^{256})}$ and $\idfun{\arrayof{\BB}}$ the identity functions on natural numbers, the storage type and byte arrays, respectively.
\end{definition}

%\begin{definition}[Code updates in execution states]
%Let the function $\updatecodeexstate{\cdot}{\cdot}{\cdot} \in \setof{\addresses} \times \exstates \times (\addresses \to \arrayof{\BB}) \to \exstates$ be defined as follows: 
%\begin{align*}
%\updatecodeexstate{s}{\addressessub}{\codeupdates} = 
%\begin{cases}
%\regstate{\mstate}{\exenv}{\updatecodegstate{\gstate}{\addressessub}{\codeupdates}} & s = \regstate{\mstate}{\exenv}{\gstate} \\
%s & \text{otherwise}
%\end{cases}
%\end{align*}
%with $\updatecodegstate{\cdot}{\cdot}{\cdot} \in  \setof{\addresses} \times \gstates \times (\addresses \to \arrayof{\BB}) \to \gstates$ as 
%\begin{align*}
%\updatecodegstate{\gstate}{\addressessub}{\codeupdates} = \\
%\lambda a. 
%\begin{cases}
%\accountstate{\nonce}{\balance}{\storage}{\codeupdates(a)} & a \in \addressessub \land \gstate(a) = \accountstate{\nonce}{\balance}{\storage}{\accountcode}\\
%\bot & a \in \addressessub \land \gstate(a) = \bot \\
%\gstate(a) & a \not \in \addressessub
%\end{cases}
%\end{align*}
%\end{definition}

%TODO how is balance defined on non existing states? This is important for the semantics here. If it is \bot as well than the call robustness definition captures that no new contracts should be created (probably useful) otherwise it would just consider changes in those accounts that already existed at the beginning.
%\end{definition}
Note that for defining call robustness, we require that depending  on the code of untrusted accounts, the effect of the contract execution should not affect the balances of the global state. This definition captures that the attacker should not be able to influence the (overall) money flows of a considered contract (as was done in the DAO hack). Still this does not consider whether the money flows were performed by the attacker directly or by invoking a  third contract (and consequently spending the attackers or the third contract's money) or if they were performed using the original contract. 
For this reason, we want to present an alternative definition for call robustness that captures this other facet of reentrancy, namely that the actions of the considered contract are influenced by untrusted code rather than its overall effect on the block chain. 
This definition is incomparable to the one before as not every different sequence of actions might result in a different effect on the balances. 

For expressing this property, we introduce the notion of substacks and to this end we first define concatenation ($++$) for plain (annotated) call stacks using a recursive definition: 
\begin{definition}[Concatenation of plain call stacks]
	\begin{align*}
	\concatstack{\nil}{\callstackplain} &= \callstackplain \\
	\concatstack{\cons{\exstate}{\callstackplain}}{\callstackplain'} &= \cons{\exstate}{(\concatstack{\callstackplain}{\callstackplain'})}
	\end{align*}
\end{definition}

Using concatenation, we define the substack relation: 
\begin{definition}[Substack]
	The plain call stack $\callstackplain$ is a (strict) substack of $\callstack$ (written $\callstackplain \subcallstack \callstack$ or $\callstackplain \subcallstackeq \callstack$ respectively) if there exists an execution state $\exstate$ and a plain call stack $\callstackplain'$ such that $\callstack = \cons{\exstate}{(\concatstack{\callstackplain'}{\callstackplain})}$. 
\end{definition}
The definition carries easily over to annotated call stacks. 

The notion of substacks helps to argue about nested calls. Given call stacks $\callstack, \callstack' \in \callstacks$ such that $\ssteps{\transenv}{\callstack}{\callstack'}$ and $\callstack \subcallstack \callstack'$ one knows that the top execution state of $\callstack$ was in the mode of calling and $\callstack'$ is a configuration within this call (before returning) as otherwise the  both call stack could not agree on their suffix. (Note that execution states are unique within an execution due to the strictly monotonically decreasing gas values). 

For completeness, we also define the independence of the locally loaded untrusted code and of return values of untrusted contract's execution: 

%For expressing the creation of arbitrary accounts
\begin{definition}[Weak update on global state]
	We define the function $\weakupdategstate{\cdot}{\cdot} \in \gstates \times\gstates \to \gstates$ that performs a weak update on global state as follows: 
	\begin{align*}
	\weakupdategstate{\gstate}{\gstate'} = 
	\lambda a. 
	\begin{cases}
	\gstate'(a) & \gstate(a) = \bot  \\
	\gstate (a) & \text{otherwise}
	\end{cases}
	\end{align*}
\end{definition}

Intuitively, when a contract $c$ should not depend on the effect of another contract, after each call to this contract, the state needs considered to be changed in an arbitrary way and the contract should be considered to return an arbitrary value. Consequently, only those contracts that produce the same traces after the the call independently of possible changes to the global state and independently of the return value that was given back can be considered independent. We, however, assume that a contract cannot arbitrarily alter the global state: Codes of existing contracts can never be changed by other contracts and in addition we assume that nonce and balance of $c$ are not touched as this would require a re-entering of the contract. 

\begin{definition}[Independence of external contract effects]
A contract $c \in \contracts$ is independent of the return values of a set of untrusted contract addresses $\untrustedaddresses$ if for all valid initial configurations $(\transenvinit, \annotate{\stateinit}{x}) \in \transenvs \times \annotatedexstates$ and all states $s, s'' \in \exstates$, all $c' \in \untrustedaddresses$ and all annotated call stacks $\callstack \in \annotatedcallstacks$ such that $\ssteps{\transenvinit}{\cons{\annotate{\stateinit}{x}}{\nil}}{\cons{\annotate{s}{c}}{\callstack}} \rightarrow \cons{\annotate{s''}{c'}}{\cons{\annotate{s}{c}}{\callstack}}$ it should hold that 
%($\exists u_\textit{stor} \in (\BB^{256} \to \BB^{256}) \to (\BB^{256} \to \BB^{256}) . u_s(c) = (\idfun{\NN}, \idfun{\NN}, u_\textit{stor}, \idfun{\arrayof{\BB}})$ and $\forall a \in \addresses \{c\}.\exists u_n \in \NN \to \NN, u_b \in \NN \to  \NN, u_\textit{stor} \in (\BB^{256} \to \BB^{256}) \to (\BB^{256} \to \BB^{256}). (u_b, u_n, u_{\textit{stor}}, \idfun{\arrayof{\BB}})$ )
for all 
$s', t' \in \potfinstates$
% changes performed on s': arbitrary weak updates + arbitrary changes in all accounts but c not effecting the codes for all weak updates and all sets and all strong update functions that map code to identity and for contract c also balance and nonce 
% What should really expressed? s' is final, so it is either EXP or Halt, if it is HALT then t' can either be EXP or HALT with different gas (but actually the gas can not be to big right? Because then after a call the execution could have more money?) and different return data. If s' is EXP then t' should not need to be EXP as well but could be also HALT, but the gstate in this case would need to have similarities to those of the caller state. Maybe it would be better not to compare s' and t' but s and t' (would help with the gstate issue), but not with the gas: one could insert a ,sanity check' in the semantics so that the semantics get stuck in this case 
%TODO care about the gas 
\begin{align*}
\sstepstrace{\transenvinit}{\cons{\annotate{s'}{c'}}{\cons{\annotate{s}{c}}{\callstack}}}{\cons{\annotate{s''}{c}}{\callstack}}{\pi} 
\land \finalstate{s''}  \\
\land \sstepstrace{\transenvinit}{\cons{\annotate{t'}{c'}}{\cons{\annotate{s}{c}}{\callstack}}}{\cons{\annotate{t''}{c}}{\callstack}}{\pi'} 
\land \finalstate{t''}  \\
\implies \project{\pi}{\filtercallscreates{c}} = \project{\pi'}{\filtercallscreates{c}}
\end{align*}
\end{definition}

where the set of potential final states $\potfinstates$ is defined as follows: 
\begin{align*}
&\potfinstates \define \\
\{ & \excstate,  \haltstate{\weakupdategstate{\strongpartialupdategstate{\globalstate(s)}{u_s}}{u_w}}{g}{d}  \\
~&|~ g \in \NN \land d \in \arrayof{\BB} \land u_w \in \sigma \\
&\land u_s  \in \strongupdategstatetype \\
&\land \exists u_\textit{bal} \in \NN.\, u_s(c) = (\idfun{\NN}, u_\textit{bal}, \idfun{(\BB^{256} \to \BB^{256}) \to (\BB^{256} \to \BB^{256})}, \idfun{\arrayof{\BB}}) \\
&\land \forall a \in \addresses / \{c\}.\exists u_n \in \NN \to \NN, u_b \in \NN \to  \NN, u_\textit{stor} \in (\BB^{256} \to \BB^{256}) \to (\BB^{256} \to \BB^{256}). \\
& \qquad \, u_s(a) = (u_b, u_n, u_{\textit{stor}}, \idfun{\arrayof{\BB}})\}
\end{align*} 

Finally, we need to capture the case that the contract might directly access untrusted code and depend on this value. To this end we introduce the notion of small steps under local update. Intuitively, this allows for accessing different codes for addresses in the global state while running a contract than those used when calling. 
\begin{definition}[Small steps under local update]
The small step relation under local (code) update $f \in \addresses \pto \arrayof{\BB}$ is recursively defined by the following rules: 
\begin{mathpar}
\infer
{ }
{\sstepslocalupdate{\transenv}{\cons{s}{\callstack}}{\cons{s}{\callstack}}{f}}

\infer
{\sstep{\transenv}{\cons{\updatecodeexstate{s}{f}}{\callstack}}{\cons{\updatecodeexstate{s'}{f}}{\callstack}} \\
\sstepslocalupdate{\transenv}{\cons{s'}{\callstack}}{\cons{s''}{\callstack}}{f} }
{\sstepslocalupdate{\transenv}{\cons{s}{\callstack}}{\cons{s''}{\callstack}}{f}}

\infer
{\sstep{\transenv}{\cons{s}{\callstack}}{\cons{s'}{\cons{s}{\callstack}}} \\
\ssteps{\transenv}{\cons{s'}{\cons{s}{\callstack}}}{\cons{s''}{\cons{s}{\callstack}}} \\
\finalstate{s''} \\
 \sstep{\transenv}{\cons{s''}{\cons{s}{\callstack}}}{\cons{s'''}{\callstack}} \\
f' = f \cup \{(a, \textit{code}) ~|~ (\globalstate(s))(a) = \bot \land
 \exists n,  b, \text{stor}.\, (\globalstate(s))(a) = (n, b, \textit{stor}, \textit{code})  \} \\
 \sstepslocalupdate{\transenv}{\cons{s'''}{\callstack}}{\cons{s''''}{\callstack}}{f'} 
}
{\sstepslocalupdate{\transenv}{\cons{s}{\callstack}}{\cons{s''''}{\callstack}}{f}}
\end{mathpar}
\end{definition}
This definition can also be easily extended to the (annotated) traces semantics. 

\begin{definition}[Local independence of untrusted code]
A contract $c \in \contracts$ is locally independent of a set of untrusted contract addresses $\untrustedaddresses$ if for all valid initial configurations $(\transenvinit, \annotate{\stateinit}{x}) \in \transenvs \times \annotatedexstates$ and all states $s \in \exstates$ and all annotated call stacks $\callstack \in \annotatedcallstacks$ such that $\ssteps{\transenvinit}{\cons{\annotate{\stateinit}{x}}{\nil}}{\cons{\annotate{s}{c}}{\callstack}}$, for all execution states $s', s'' \in \exstate$, for all $f \in \addresses \pto \arrayof{\BB}$ with $\domain{f} = \untrustedaddresses$
\begin{align*}
\sstepstrace{\transenvinit}{\cons{\annotate{s}{c}}{\callstack}}{\cons{\annotate{s'}{c}}{\callstack}}{\pi}
~\land~ \finalstate{s'} \\
~\land~ \sstepslocalupdatetrace{\transenvinit}{\cons{\annotate{s}{c}}{\callstack}}{\cons{\annotate{s''}{c}}{\callstack}}{f}{\pi'}
~\land~ \finalstate{s''} \\
\implies \project{\pi}{\filtercallscreates{c}} = \project{\pi'}{\filtercallscreates{c}}
\end{align*}
\end{definition}

In addition, we define balance equality on final execution states: 
\begin{definition}[Balance equality on final execution states]
Two final execution states $s, s' \in \exstates$ are equal with respect to the balances ($s \equalonbalances s'$) if for some global states $\gstate, \gstate\ \in \gstates$ and some gas values $\lgas, \lgas' \in \NN$ and some output data $d, d' \in \arrayof{\BB}$ one of the following holds: 
\begin{enumerate}
\item  $s = s' = \excstate$ 
\item 
$\exstate = \haltstate{\gstate}{\lgas}{c} 
\land \exstate' = \haltstate{\gstate'}{\lgas'}{d'}$ \\
$\land \forall \contractaddress \in \addresses. \, \balance \,(\gstate \, (\contractaddress)) = \balance \, (\gstate' \, (\contractaddress))$
\end{enumerate}
\end{definition}

We define independence of (parts of) the transaction environment as this can be influenced by miners.
Intuitively, the effects a contract execution has on the flow of money should not be affected by (previously specified) components of the transaction environment. 

We assume $\transenvcomponents$ to be the set of the accessor functions of the transaction environment. 
We define the equality up to a component for transaction environments:
\begin{definition}[Equality up to components]
Two transaction environments $\transenv$, $\transenv'$ are equal upto component $\transenvcomponent \in \transenvcomponents$ (written $\transenv \equalupto{\transenvcomponent} \transenv'$) if 
\begin{align*}
\forall \transenvcomponent' \in \transenvcomponents / \{ \transenvcomponent \}. \; \transenvcomponent'(\transenv) = \transenvcomponent'(\transenv')
\end{align*}
\end{definition}

\begin{definition}
A contract $c$ is independent of a subset $I \subseteq \transenvcomponents$ of components of the transaction environment if for all $\transenvcomponent \in I$, for all valid initial configurations $(\transenvinit, \annotate{\stateinit}{x}) \in \transenvs \times \annotatedexstates$ and all states $s \in \exstates$ and all annotated call stacks $\callstack \in \annotatedcallstacks$ such that $\ssteps{\transenvinit}{\cons{\annotate{\stateinit}{x}}{\nil}}{\cons{\annotate{s}{c}}{\callstack}}$ for all $\transenv \in \transenvs$ the following condition holds: 
\begin{align*}
& \transenvcomponent(\transenvinit) \neq \transenvcomponent(\transenv) 
\land \transenvinit \equalupto{\transenvcomponent} \transenv \\ 
&\land \ssteps{\transenvinit}{\cons{\annotate{\exstate}{c}}{\callstack}}{\cons{\annotate{\exstate'}{c}}{\callstack}} 
~\land~ \ssteps{\transenv}{\cons{\annotate{\exstate}{c}}{\callstack}}{\cons{\annotate{\exstate''}{c}}{\callstack}} \\ 
& \land  \finalstate{\exstate'} 
\land \finalstate{\exstate''} 
\implies \exstate' \equalonbalances \exstate''
\end{align*}
\end{definition}

\subsection{Call restriction}
Even though the Solidity syntax conveys the impression of being able to communicate with well-defined contract instances, this is not necessarily the case. If a contract shall interact with an already existing contract on the blockchain, the developer needs to specify the address of this contract or the contract address needs to be derived dynamically from the context. Both these approaches are error-prone and may lead to money transfers or to code executions that were not intended by the user. 

Consider the following example: 
\begin{lstlisting}
contract FriendlyMoney { 
	address friend = 0xBa8AA02Fec8d3D440B3A1B60edDAAD80521581c9; 
	
	function sendMoneyToMyFriend(uint amount){ 
		DonateMeMoney(friend).donate(amount); 
	}
}
\end{lstlisting}
Specifying that a contract is an instance of a certain class (as done by \lstinline|DonateMeMoney(friend)|) does not imply any run time checks, but only facilitates the calling of its functions. If at the specified address no contract of the of the specified form can be found, the callback function of the account at this address will be executed. Consequently, giving a wrong \lstinline|friend| address might not only result in sending money to the wrong account, but also in executing untrusted code. 

%These considerations highlight the tricky nature of Solidity semantics and motivate the importance of a precise semantic model for rigorous security reasoning. 

In order to prevent such undesired effects, a user should be able to specify the set of contract addresses it expects to perform calls to. We introduce a property which we call \emph{call restriction} that ensures that only the a predefined set of desired contracts is entered during execution.

\begin{definition}[Call restriction]
A contract $c \in \contracts$ restricts calls to a set of addresses $\callableaddresses \subseteq \addresses$ 
if for all reachable configurations $(\transenv, \cons{\annotate{s}{c}}{\callstack})$ it holds that 
\begin{align*}
\ssteps{\transenv}{\cons{\annotate{\exstate}{c}}{\callstack}}{\cons{\annotate{\exstate'}{c'}}{\concatstack{\callstack'}{\cons{\annotate{\exstate}{c}}{A}}}} 
\implies \getcontractaddress{c'} \in \callableaddresses 
\end{align*}
\end{definition}

A more liberal version of this property might require that contracts outside the call set might be called, but only if they do not perform any modifications on the global state (so basically they don't have side effects). 
A potential use case of this definition might be a contract only calling library functions for computations. 

\TODOC{For this we do not have a proper motivating example. My idea was something that one would like to ensure that only libraries for computations are used or something similar. But I am not sure whether I like to property too much, but it's a trace property}
\begin{definition}[Relaxed call restriction]
A contract $c \in \contracts$ restricts calls to a set of addresses $\callableaddresses \subseteq \addresses$ and only performs side-effectless calls otherwise 
if for all reachable configurations $(\transenv, \cons{\annotate{s}{c}}{\callstack})$ it holds for all $c' \not \in \callableaddresses$ that
\begin{align*}
\ssteps{\transenv}{\cons{\annotate{\exstate}{c}}{\callstack}}{\cons{\annotate{\exstate'}{c'}}{\concatstack{\callstack'}{\cons{\annotate{s}{c}}{\callstack}}}} \rightarrow^* \cons{\annotate{\exstate''}{c'}}{\concatstack{\callstack'}{\cons{\annotate{s}{c}}{\callstack}}} 
~\land~ \finalstate{s''} \\
\implies s'' = \excstate ~\lor~ s'' = \haltstatefull{\gstate}{d}{g}{\transeffects} ~\land~ \forall a \in \callableaddresses . \, (\globalstate(s'))(a) = \gstate(a)
\end{align*}
\end{definition}

%\begin{definition}[Relaxed call restriction]
%A contract $c$ restricts calls to a set $\callableaddresses$ of addresses and only performs side-effectless calls otherwise if for all valid initial configurations $(\transenvinit, \annotate{\stateinit}{x}) \in \transenvs \times \annotatedexstates$ and all states $s \in \exstates$ and all annotated call stacks $\callstack \in \annotatedcallstacks$ such that $\ssteps{\transenvinit}{\cons{\annotate{\stateinit}{x}}{\nil}}{\cons{\annotate{s}{c}}{\callstack}}$, for all $c' \not \in \callableaddresses$, $\callstack' \in \annotatedcallstacks$ and $s',s'' \in \exstates$ the following condition holds:
%\begin{align*}
%\ssteps{\transenvinit}{\cons{\annotate{\exstate}{c}}{\callstack}}{\cons{\annotate{\exstate'}{c'}}{\callstack'}} 
%~\land~ \cons{\annotate{s}{c}}{\callstack} \subcallstackeq \callstack' \\
%~\land~ \ssteps{\transenvinit}{\cons{\annotate{\exstate'}{c'}}{\callstack'}}{\cons{\annotate{\exstate''}{c'}}{\callstack'}}
%~\land~ \finalstate{s''} \\
%\implies s'' = \excstate ~\lor~ s'' = \haltstate{\gstate}{d}{g} ~\land~ \forall a \in \callableaddresses . \, (\globalstate(s'))(a) = \gstate(a)
%\end{align*}
%\end{definition}

%TODO some lemma to relate with call robustness? 

\subsubsection{Securify}
Recently, the online tool Securify \cite{securify} has been presented at the third Ethereum Foundation Developers conference on November 1-4 2017.  Securify supports automated checks for transaction reorder dependency, reentrancy, some insecure coding patterns and some more specific properties as checking whether a contract locks Ether and a version of miner dependency that checks whether influenceable data is used as input to the SHA3 function. The authors of Securify claim that the tool provides 'guarantees, to avoid reporting vulnerable contracts are safe'.

%In order for an static analysis tool for EVM byte code to provide reliable guarantees, two prerequisites need to be given: 
%\begin{enumerate}
%\item 
%A cleanly defined concrete semantics for the EVM
%\item 
%A formal characterization of the security properties that should not be violated (expressed in terms of the concrete semantics)
%\end{enumerate}
%Only in the presence of those two components, it can be expressed (and proven) that a certain behavior detected in the analysis implies the satisfaction of a security property in the concrete execution of the contract. 

In the case of Securify, we unfortunately could not find any work published on the underlying theory so far, so that we were only able to evaluate their tool for checking the soundness claim. We came to the conclusion that either the underlying abstraction they perform cannot be sound or that the security patterns that they use for characterizing good behavior are not sufficient. 

For example, they report the example from Figure~\ref{exc_fn} not to contain mishandled exceptions. 
For transaction order dependency, they seem to follow a more advanced approach than Oyente, but still the following example is wrongly classified as independent of transaction ordering: 

\lstinputlisting{tod_fn_securify.sol}

This contract clearly is transaction order dependent as only the first transaction calling the \lstinline|payoutMoney| functions receives the payout that is sent in the initialization code of the \lstinline|Dummy| contract created in the function.
